# Supplementary material for: Rewriting or Reweighting? A Geometric Account in Language Models
Source: arXiv:2608.01835 source file (2026-08-03)
Supplement: Supplementary file 1 [file sections__appendix_tables.tex]

\section{Appendix: Full Numerical Summaries}
\label{sec:appendix_tables}

\subsection{Cross-Model Repetition Strength}
Table~\ref{tab:rep_strength_act} gives representative ACT-space repetition strength measurements.  The full CSV files are included in the repository under \texttt{data__}.  $T_{base}$ is the baseline repetition tendency at $\alpha=1$; $N_R$ is the number of selected R-Neurons; $N_R^{eff}$ is the PCA dimension at the $90\%$ variance threshold.

\begin{table*}[h]
\centering
\small
\begin{tabular}{lrrrrr}
\toprule
Model & $G^{uniF}_{ACT}$ & $G^{occ}_{ACT}$ & $G^{causal}$ & $T_{base}$ & $N_R^{eff}$ \\
\midrule
Gemma-2-2B & 6.8465 & 0.9809 & 0.2942 & 0.8632 & 13 \\
Gemma-2-2B-it & 8.0945 & 0.7189 & 0.2750 & 0.6800 & 15 \\
Qwen2.5-0.5B & 7.5528 & 0.7049 & 0.2108 & 0.8562 & 26 \\
Qwen2.5-0.5B-Instruct & 7.1556 & 0.7323 & 0.5994 & 0.8219 & 25 \\
Mistral-7B-v0.3 & 10.3875 & 0.6061 & 0.1661 & 0.8833 & 25 \\
Mistral-7B-Instruct & 8.3211 & 0.6757 & 0.2480 & 0.8713 & 18 \\
Llama-3.1-8B & 3.6277 & 1.1152 & 0.0891 & 0.9082 & 9 \\
Llama-3.1-8B-Instruct & 4.3802 & 1.1844 & 0.1823 & 0.7599 & 8 \\
\bottomrule
\end{tabular}
\caption{Representative repetition strength measurements in ACT space.}
\label{tab:rep_strength_act}
\end{table*}

\subsection{Sycophancy Low-Rank Statistics}
Table~\ref{tab:syco_lowrank_appendix} summarizes selected sycophancy PCA results.  ACT-space PC1 explained variance is usually larger than NOC-space PC1 explained variance, suggesting that the runtime sycophancy state is more concentrated than the functional contribution basis.

\begin{table*}[h]
\centering
\small
\begin{tabular}{lrrrr}
\toprule
Model & NOC PC1 & NOC Dim90 & ACT PC1 & ACT Dim90 \\
\midrule
Qwen2.5-0.5B & 0.2025 & 38 & 0.6011 & 4 \\
Qwen2.5-7B & 0.2924 & 28 & 0.7673 & 3 \\
Qwen2.5-32B & 0.2603 & 32 & 0.7952 & 3 \\
Gemma-2-27B-it & 0.2919 & 23 & 0.6587 & 2 \\
Llama-3.1-8B & 0.3093 & 29 & 0.4262 & 8 \\
Mistral-Nemo-Instruct & 0.2799 & 25 & 0.6764 & 6 \\
\bottomrule
\end{tabular}
\caption{Selected sycophancy low-rank statistics in NOC and ACT spaces.}
\label{tab:syco_lowrank_appendix}
\end{table*}

\subsection{Placeholders for Final Submission}
The following tables should be filled before submission.

\begin{table}[h]
\centering
\small
\begin{tabular}{lccc}
\toprule
Experiment & Repetition & Sycophancy & Status \\
\midrule
Behavior-mismatch steering & TBD & TBD & Planned \\
Transfer steering & TBD & TBD & Planned \\
Iso-behavior geometry & TBD & TBD & Planned \\
Qwen/Gemma replication & TBD & TBD & Planned \\
Layer-wise atlas & TBD & TBD & Optional \\
\bottomrule
\end{tabular}
\caption{Open experimental slots.}
\label{tab:open_slots}
\end{table}
