# Supplementary material for: Rewriting or Reweighting? A Geometric Account in Language Models
Source: arXiv:2608.01835 source file (2026-08-03)
Supplement: Supplementary file 2 [file supplementary.tex]

\documentclass[letterpaper,twocolumn]{article}
\usepackage[submission]{aaai2027}
\usepackage{natbib}
\usepackage{graphicx}
\usepackage{amsmath,amssymb,mathtools}
\usepackage{booktabs}
\usepackage{multirow}
\usepackage{array}
\usepackage{adjustbox}
\usepackage{tabularx}
\usepackage{makecell}
\usepackage{xcolor}
\usepackage{enumitem}
\usepackage{url}
\usepackage{pifont}
\newcommand{\ACT}{\mathrm{ACT}}
\newcommand{\CETT}{\mathrm{CETT}}
\newcommand{\R}{\mathbb{R}}
\newcommand{\E}{\mathbb{E}}
\newcommand{\Cov}{\mathrm{Cov}}
\newcommand{\tr}{\mathrm{tr}}
\newcommand{\diag}{\mathrm{diag}}
\newcommand{\logit}{\mathrm{logit}}
\DeclareMathOperator{\corr}{corr}
\providecommand{\BAC}{\textsc{bac}}
\providecommand{\BACs}{\textsc{bac}s}
\setcounter{secnumdepth}{2}
\title{%
\fontsize{17pt}{20pt}\selectfont
Supplementary Material:\\
Rewriting or Reweighting? A Geometric Account of Repetition and\\
Sycophancy in Language Models}
\author{Anonymous Authors}
\affiliations{}
\begin{document}
\maketitle
\appendix
\end{document}
